# Supplementary material for: Memory-Efficient Optical Flow via Radius-Distribution Orthogonal Cost Volume
Source: arXiv:2312.03790 source file (2025-03-04)
Supplement: Supplementary file 1 [file X_suppl.tex]

\clearpage
\setcounter{page}{1}
\maketitlesupplementary

\begin{table}
  \centering
%   \small
%   \setlength{\tabcolsep}{3.pt}
  \begin{tabular}{l|cccc}
    \toprule
    \multirow{2}{*}{Method} & \multicolumn{4}{c}{KITTI 2012 (Reflective)} \\
    & 3-noc & 3-all &4-noc &4-all \\
    \midrule
    BGNet+~\cite{bgnet} & 6.44 & 8.41 & 4.26 & 5.80 \\
    AANet+~\cite{aanet} & 7.22 & 9.10 & 5.25  & 6.66 \\
    CoEx~\cite{coex} & 6.83 & 8.63 & 4.61 & 6.00 \\
    Fast-ACVNet+~\cite{fast-acv} & 6.82 & 8.59 & 4.83 & 6.06 \\
    HITNet~\cite{hitnet} & 5.91 & 7.54 & 4.04 & 5.34 \\
    \midrule
    w/o BA (2D) & 8.81 & 10.61 & 6.17 & 7.63 \\
    BANet-2D & \underline{5.59} & \underline{7.27} & \underline{3.77} & \underline{5.08} \\
    \midrule
    w/o BA (3D) & 6.10 & 8.06 & 4.14 & 5.63 \\
    BANet-3D & \textbf{5.37} & \textbf{7.07} & \textbf{3.64} & \textbf{4.89} \\
    \bottomrule
  \end{tabular}
  \caption{Quantitative evaluation in reflective (ill-posed) regions of the KITTI 2012 test set.} 
  \label{tab:reflective}
\end{table}

\begin{figure}
\centering
{\includegraphics[width=1.0\linewidth]{./figures/supp_v1_v2.pdf}}
\caption{Qualitative comparisons with MobileStereoNet-2D~\cite{mobilestereonet} on the test set of KITTI 2015~\cite{kitti2015}. Significant improvements are highlighted by white dashed boxes. Our
bilateral aggregation produces clear edges and preserves intricate details. Zoom in for a clearer view.}
\label{fig:supp_v1}
\end{figure}

\begin{figure}
\centering
{\includegraphics[width=1.0\linewidth]{./figures/supp_v2.pdf}}
\caption{Visual results of the detailed aggregation branch, the smooth aggregation branch, and the final prediction.}
\label{fig:supp_v2}
\end{figure}

\section{More Experimental Results}

\subsection{Performance in Reflective Regions}
To verify the performance of our bilateral aggregation (BA) in smooth regions, such as reflective regions. 
We compared our approach with previously published real-time methods (on high-end GPUs) as well as our baseline method, which removes the bilateral aggregation (denoted as w/o BA). The comparison results are presented in \cref{tab:reflective}, where our BANet-3D achieves the best performance. Compared to other methods, our bilateral aggregation can adaptively separate the full cost volume into detailed and smooth cost volumes. This enables the smooth aggregation network to specialize in learning to handle smooth regions, including reflective regions. As a result, our method outperforms previous approaches by a significant margin in reflective regions. 

Specifically, compared to the baseline (w/o BA), our bilateral aggregation (BA) achieves a significant improvement, such as a 36.5\% improvement for 2D convolution-based aggregation networks and a 12.0\% improvement for 3D convolution-based ones.

\subsection{More Qualitative Comparisons}
As shown in \cref{fig:supp_v1}, we provide more visual comparisons with MobileStereoNet-2D~\cite{mobilestereonet}. Both MobileStereoNet-2D and our BANet-2D rely solely on 2D convolutions, avoiding costly 3D convolutions or operations that are unfriendly to mobile devices. MobileStereoNet-2D struggles to simultaneously handle high-frequency edges and details, and low-frequency smooth regions, resulting in blurred edges and loss of fine details. In comparison, our method effectively addresses these challenges by the proposed bilateral aggregation. As a result, our approach produces clear edges and preserves intricate details.

\subsection{Detailed and Smooth Visual Results}
\cref{fig:supp_v2} shows visual results of the detailed aggregation branch, the smooth aggregation branch, and the final prediction. The smooth aggregation branch performs well in handling low-frequency smooth regions but struggles with high-frequency edges and details, as indicated by the white dashed boxes in \cref{fig:supp_v2}. In contrast, the detailed aggregation branch excels at handling high-frequency edges and details but underperforms in low-frequency smooth regions. Our final prediction combines the strengths of both branches, effectively addressing high-frequency edges and details while also handling low-frequency smooth regions.
